# Supplementary material for: Diffusion Model Driven Test-Time Image Adaptation for Robust Skin Lesion Classification
Source: arXiv:2405.11289 source file (2024-05-18)
Supplement: Supplementary file 1 [file Supplementary.tex]

% % This is samplepaper.tex, a sample chapter demonstrating the
% % LLNCS macro package for Springer Computer Science proceedings;
% % Version 2.20 of 2017/10/04
% %
% \documentclass[runningheads]{llncs}
% \usepackage{graphicx}
% \usepackage[utf8]{inputenc} % allow utf-8 input
% \usepackage{hyperref}       % hyperlinks
% \usepackage{url}            % simple URL typesetting
% \usepackage{booktabs}       % professional-quality tables
% \usepackage{amsfonts}       % blackboard math symbols
% \usepackage{nicefrac}       % compact symbols for 1/2, etc.
% \usepackage{microtype}      % microtypography
% \usepackage{xcolor}         % colors
% \usepackage{cite}
% \usepackage{color,colortbl}
% \usepackage{subcaption}
% \usepackage{adjustbox}
% \usepackage{multirow}
% \usepackage{amsmath}
% \usepackage{algorithm}      % 用于算法的浮动环境
% \usepackage{algpseudocode}  % 用于算法的伪代码
% \usepackage{amsmath}        % 提供数学命令和环境

% \usepackage{caption}
% \usepackage[percent]{overpic}
% \usepackage{enumitem}
% \usepackage{graphicx}
% \setlength{\intextsep}{10pt plus 2pt minus 2pt}
% \usepackage{subcaption}

% \newcommand{\ie}{i.e.,}
% \DeclareMathOperator*{\argmax}{arg\,max}
% % Used for displaying a sample figure. If possible, figure files should
% % be included in EPS format.
% %
% % If you use the hyperref package, please uncomment the following line
% % to display URLs in blue roman font according to Springer's eBook style:
% % \renewcommand\UrlFont{\color{blue}\rmfamily}


% \begin{document}
% %
% % \title{Contribution Title\thanks{Supported by organization x.}}
% \title{Appendix for ``Diffusion Model Driven Test-Time Image Adaptation for Robust Skin Lesion Classification"}

% %
% %\titlerunning{Abbreviated paper title}
% % If the paper title is too long for the running head, you can set
% % an abbreviated paper title here
% %
% % \author{First Author\inst{1}\orcidID{0000-1111-2222-3333} \and
% % Second Author\inst{2,3}\orcidID{1111-2222-3333-4444} \and
% % Third Author\inst{3}\orcidID{2222--3333-4444-5555}}
% % %
% % \authorrunning{F. Author et al.}
% % % First names are abbreviated in the running head.
% % % If there are more than two authors, 'et al.' is used.
% % %
% % \institute{Princeton University, Princeton NJ 08544, USA \and
% % Springer Heidelberg, Tiergartenstr. 17, 69121 Heidelberg, Germany
% % \email{lncs@springer.com}\\
% % \url{http://www.springer.com/gp/computer-science/lncs} \and
% % ABC Institute, Rupert-Karls-University Heidelberg, Heidelberg, Germany\\
% % \email{\{abc,lncs\}@uni-heidelberg.de}}

% % \author{Anonymous}
% % \institute{}
% % \maketitle              % typeset the header of the contribution

% % \section{Common Corruptions}
% % Gaussian noise, often seen in conditions of low lighting, represents the first type of corruption. In the presence of minimal light, this type of disturbance can manifest. Another form of corruption, known as shot noise or Poisson noise, arises from the inherent randomness of light, leading to electronic noise. Similar to salt-and-pepper noise but in color, impulse noise can emerge from bit errors. When the focus is not accurately set, defocus blur makes the image appear blurry. The effect of Frosted Glass Blur is akin to looking through frosted glass windows or panels. Motion blur is observed when the camera is in rapid movement. Rapidly moving towards an object can induce zoom blur. The intensity of daylight influences brightness levels. Depending on the lighting and the colors of the object being photographed, contrast can vary between high and low. Elastic transformations involve the stretching or contracting of small regions within an image. Pixelation is a result of enlarging a low-resolution image. Lastly, JPEG, known for being a lossy compression format, can introduce compression artifacts into images.
% % Table generated by Excel2LaTeX from sheet 'Sheet1'

% % \begin{figure}[t]
% % \centering
% % \begin{overpic}[width=1\textwidth]{fig/isic_ge.pdf}
% % \end{overpic}
% % \caption{.}
% % \label{fig:isic_ge}
% % % \vspace{-0.55 cm}
% % \end{figure}

% % \begin{figure}[ht!]
% %     \centering
% %     \includegraphics[width=0.63\linewidth]{fig/isic_ge1.pdf}
% %     \hspace*{0.09cm}
% %     \includegraphics[width=0.65\linewidth]{fig/isic_ge2.pdf}
% %     \caption{Some generated examples, \textbf{left:} original image, \textbf{middle:} corrupted image, \textbf{right:} generated image.}
% % \end{figure}

% % \begin{figure}[b!]
% % \centering
% % \begin{overpic}[width=0.65\textwidth]{fig/level.pdf}
% % \end{overpic}
% % \caption{Examples of different corruptions at five different severity levels.}
% % \end{figure}

% % \begin{figure}[ht!]
% %     \centering
% %     \captionsetup{skip=5pt}
% %     \includegraphics[width=0.55\textwidth]{fig/level.pdf}
% %     \caption{Examples of different corruptions at five different severity levels.}
% %     \vspace{0.1cm} 
% %     \includegraphics[width=0.57\linewidth]{fig/isic_ge1.pdf}
% %     % \caption{Some generated examples, \textbf{left:} original image, \textbf{middle:} corrupted image, \textbf{right:} generated image.}
% %     \vspace{0.1cm} % Adjust vertical spacing between figures as needed
% %     \includegraphics[width=0.592\linewidth]{fig/isic_ge2.pdf}
% %     \hspace*{-0.295cm}
% %     \caption{Some generated examples, \textbf{left:} original image, \textbf{middle:} corrupted image, \textbf{right:} generated image.}
% % \end{figure}
% \begin{figure}[ht!]
%     \centering
%     \captionsetup{skip=5pt}
%     \includegraphics[width=0.65\textwidth]{fig/level.pdf}
%     \caption{Examples of different corruptions at five different severity levels.}
%     \vspace{0.1cm} 
%     \includegraphics[width=0.65\linewidth]{fig/isic_ge1.pdf}
%     % \caption{Some generated examples, \textbf{left:} original image, \textbf{middle:} corrupted image, \textbf{right:} generated image.}
%     \vspace{0.1cm} % Adjust vertical spacing between figures as needed
%     \includegraphics[width=0.677\linewidth]{fig/isic_ge2.pdf}
%     \hspace*{-0.425cm}
%     \vspace{-0.5cm} % Adjust vertical spacing between the last figure and caption
%     \caption{Some generated examples, \textbf{left:} original image, \textbf{middle:} corrupted image, \textbf{right:} generated image.}
% \end{figure}



% \begin{table}[t!]
%   \tiny
%   \centering
%   \caption{Results of all corruptions and classifiers on the ISIC2019-C dataset.}
%     \begin{tabular}{l|c|ccc|ccc|ccc|}
%           & \multicolumn{1}{c}{} & \multicolumn{3}{p{12.57em}}{ResNet-50} & \multicolumn{3}{p{12.57em}}{Swin-T} & \multicolumn{3}{p{12.57em}}{ConvNeXt-T} \\
% \cmidrule{2-11}          & \multicolumn{1}{p{5.5em}|}{Corruption level} & \multicolumn{1}{p{4.19em}}{Corrupted} & \multicolumn{1}{p{4.19em}}{~~DDA} & \multicolumn{1}{p{4.19em}|}{~~Ours} & \multicolumn{1}{p{4.19em}}{Corrupted} & \multicolumn{1}{p{4.19em}}{~~DDA} & \multicolumn{1}{p{4.19em}|}{~~Ours} & \multicolumn{1}{p{4.19em}}{Corrupted} & \multicolumn{1}{p{4.19em}}{~~DDA} & \multicolumn{1}{p{4.19em}|}{~~Ours} \\
%     \midrule
%     \multicolumn{1}{p{8.44em}|}{original} & 0     & \multicolumn{3}{c|}{66.54 } & \multicolumn{3}{c|}{71.20 } & \multicolumn{3}{c|}{73.29 } \\
%     \midrule
%     \multicolumn{1}{l|}{\multirow{5}[2]{*}{defocus blur}} & 1     & 66.52  & 66.50  & 66.25  & 69.42  & 69.90  & 70.07  & 72.03  & 72.54  & 72.93  \\
%           & 2     & 65.75  & 66.15  & 66.25  & 67.71  & 68.99  & 69.38  & 71.85  & 71.91  & 72.14  \\
%           & 3     & 64.59  & 64.79  & 64.92  & 65.56  & 67.02  & 67.63  & 70.05  & 70.63  & 71.04  \\
%           & 4     & 63.78  & 64.06  & 64.27  & 64.47  & 65.42  & 66.25  & 68.53  & 69.48  & 69.80  \\
%           & 5     & 63.39  & 63.74  & 63.98  & 62.97  & 63.58  & 63.94  & 66.70  & 67.25  & 68.02  \\
%     \midrule
%     \multicolumn{1}{l|}{\multirow{5}[2]{*}{glass blur}} & 1     & 66.46  & 66.29  & 66.15  & 70.78  & 71.02  & 70.31  & 72.44  & 72.99  & 72.89  \\
%           & 2     & 66.05  & 66.11  & 66.09  & 69.52  & 70.09  & 69.97  & 72.18  & 72.76  & 72.72  \\
%           & 3     & 65.40  & 65.61  & 65.69  & 68.75  & 69.22  & 69.58  & 71.87  & 71.95  & 72.14  \\
%           & 4     & 64.81  & 65.06  & 65.08  & 67.65  & 68.18  & 68.67  & 71.06  & 71.36  & 71.51  \\
%           & 5     & 64.02  & 64.00  & 64.31  & 65.69  & 66.42  & 66.68  & 69.15  & 69.90  & 70.35  \\
%     \midrule
%     \multicolumn{1}{l|}{\multirow{5}[2]{*}{motion blur}} & 1     & 66.50  & 66.42  & 66.25  & 70.59  & 70.41  & 70.05  & 72.66  & 73.23  & 73.13  \\
%           & 2     & 66.13  & 66.32  & 66.42  & 69.07  & 69.48  & 69.78  & 72.05  & 72.42  & 72.50  \\
%           & 3     & 65.26  & 65.44  & 65.42  & 67.61  & 68.40  & 68.57  & 71.06  & 71.69  & 71.51  \\
%           & 4     & 64.37  & 64.71  & 65.08  & 66.29  & 66.94  & 67.45  & 69.30  & 69.82  & 70.07  \\
%           & 5     & 63.90  & 64.17  & 64.23  & 65.56  & 66.19  & 66.07  & 67.90  & 68.46  & 68.97  \\
%     \midrule
%     \multicolumn{1}{l|}{\multirow{5}[2]{*}{zoom blur}} & 1     & 66.31  & 66.54  & 66.60  & 70.70  & 70.57  & 69.99  & 73.03  & 72.95  & 73.25  \\
%           & 2     & 65.93  & 66.23  & 66.19  & 69.97  & 70.31  & 69.64  & 72.50  & 72.58  & 72.87  \\
%           & 3     & 65.59  & 65.67  & 65.63  & 69.01  & 69.24  & 68.53  & 71.97  & 71.95  & 72.05  \\
%           & 4     & 64.88  & 65.34  & 65.36  & 68.34  & 68.97  & 68.42  & 71.41  & 72.01  & 72.12  \\
%           & 5     & 64.23  & 64.59  & 64.67  & 67.82  & 68.14  & 67.17  & 70.33  & 70.68  & 70.27  \\
%     \midrule
%     \multicolumn{1}{l|}{\multirow{5}[2]{*}{gaussian blur}} & 1     & 66.48  & 66.34  & 66.40  & 70.90  & 71.20  & 71.24  & 72.95  & 73.11  & 73.21  \\
%           & 2     & 65.95  & 66.32  & 66.32  & 68.34  & 69.42  & 69.80  & 72.01  & 72.30  & 72.34  \\
%           & 3     & 64.55  & 64.73  & 65.24  & 66.03  & 67.51  & 67.88  & 70.25  & 70.94  & 71.55  \\
%           & 4     & 63.90  & 64.35  & 64.49  & 64.47  & 65.95  & 66.56  & 69.13  & 69.46  & 69.86  \\
%           & 5     & 62.91  & 63.33  & 63.13  & 61.77  & 62.60  & 62.62  & 65.16  & 66.05  & 66.60  \\
%     \midrule
%     \multicolumn{1}{l|}{\multirow{5}[2]{*}{elastic transform}} & 1     & 67.05  & 66.80  & 66.44  & 70.90  & 70.66  & 70.43  & 72.38  & 72.66  & 72.38  \\
%           & 2     & 65.54  & 65.54  & 65.30  & 70.45  & 70.03  & 70.43  & 70.61  & 70.57  & 70.70  \\
%           & 3     & 66.64  & 66.68  & 66.13  & 71.12  & 71.10  & 70.51  & 72.87  & 73.13  & 72.83  \\
%           & 4     & 66.88  & 66.70  & 66.27  & 71.10  & 71.24  & 70.47  & 73.07  & 73.05  & 72.60  \\
%           & 5     & 66.62  & 66.58  & 66.40  & 71.34  & 71.28  & 70.37  & 72.68  & 72.83  & 72.36  \\
%     \midrule
%     \multicolumn{1}{l|}{\multirow{5}[2]{*}{jpeg compression}} & 1     & 66.23  & 65.93  & 65.69  & 69.52  & 68.61  & 67.63  & 70.29  & 70.53  & 70.15  \\
%           & 2     & 66.21  & 65.87  & 65.50  & 67.27  & 66.86  & 65.79  & 69.21  & 69.48  & 69.26  \\
%           & 3     & 65.61  & 65.50  & 65.30  & 65.81  & 64.86  & 64.21  & 67.37  & 67.45  & 67.57  \\
%           & 4     & 62.56  & 62.81  & 62.85  & 60.78  & 59.62  & 58.67  & 61.71  & 62.26  & 62.30  \\
%           & 5     & 56.72  & 56.95  & 57.03  & 55.81  & 55.45  & 55.47  & 57.57  & 57.80  & 58.10  \\
%     \midrule
%     \multicolumn{1}{l|}{\multirow{5}[2]{*}{pixelate}} & 1     & 66.60  & 66.46  & 66.15  & 71.32  & 71.24  & 70.51  & 73.41  & 73.68  & 73.60  \\
%           & 2     & 66.58  & 66.54  & 66.40  & 71.49  & 71.09  & 70.65  & 73.41  & 73.45  & 73.19  \\
%           & 3     & 66.38  & 66.29  & 65.95  & 70.88  & 71.04  & 70.86  & 72.83  & 73.09  & 73.13  \\
%           & 4     & 66.38  & 66.42  & 66.29  & 70.45  & 70.63  & 69.92  & 72.50  & 73.15  & 72.95  \\
%           & 5     & 66.76  & 66.56  & 66.30  & 61.49  & 68.12  & 70.41  & 70.23  & 71.87  & 72.82  \\
%     \midrule
%     \multicolumn{1}{l|}{\multirow{5}[2]{*}{gaussian noise}} & 1     & 57.82  & 60.74  & 62.83  & 64.00  & 67.75  & 69.40  & 69.50  & 70.49  & 71.20  \\
%           & 2     & 45.73  & 51.98  & 57.15  & 59.16  & 64.21  & 68.14  & 64.15  & 66.46  & 68.87  \\
%           & 3     & 30.70  & 38.17  & 43.95  & 54.72  & 61.00  & 65.26  & 57.68  & 61.65  & 64.51  \\
%           & 4     & 25.80  & 25.61  & 26.26  & 51.53  & 54.46  & 61.14  & 50.96  & 56.07  & 60.07  \\
%           & 5     & 24.54  & 21.88  & 19.31  & 50.68  & 51.69  & 55.59  & 49.38  & 51.77  & 54.65  \\
%     \midrule
%     \multicolumn{1}{l|}{\multirow{5}[2]{*}{impulse noise}} & 1     & 55.16  & 59.14  & 62.06  & 64.67  & 67.41  & 68.71  & 68.34  & 69.84  & 70.45  \\
%           & 2     & 40.52  & 49.12  & 54.90  & 60.41  & 64.39  & 66.36  & 62.97  & 65.65  & 67.67  \\
%           & 3     & 31.86  & 39.67  & 46.22  & 57.23  & 61.91  & 64.96  & 58.81  & 62.28  & 64.63  \\
%           & 4     & 23.08  & 24.03  & 25.96  & 52.30  & 56.60  & 60.60  & 50.70  & 55.59  & 59.32  \\
%           & 5     & 21.38  & 20.12  & 18.84  & 50.72  & 52.42  & 55.93  & 48.85  & 51.33  & 55.18  \\
%     \midrule
%     \multicolumn{1}{l|}{\multirow{5}[2]{*}{shot noise}} & 1     & 52.54  & 57.45  & 61.18  & 61.77  & 65.95  & 69.17  & 66.62  & 68.97  & 70.63  \\
%           & 2     & 38.19  & 45.63  & 51.49  & 57.76  & 61.98  & 66.46  & 61.31  & 64.57  & 67.07  \\
%           & 3     & 29.37  & 32.51  & 37.03  & 54.78  & 58.61  & 63.41  & 55.49  & 59.14  & 62.68  \\
%           & 4     & 27.26  & 24.76  & 21.90  & 52.20  & 55.38  & 58.87  & 49.89  & 53.86  & 56.86  \\
%           & 5     & 28.03  & 22.27  & 18.86  & 51.17  & 53.28  & 54.94  & 49.32  & 52.00  & 53.46  \\
%     \midrule
%     \multicolumn{1}{l|}{\multirow{5}[2]{*}{speckle noise}} & 1     & 55.02  & 59.76  & 62.38  & 63.25  & 66.52  & 68.89  & 68.38  & 70.11  & 70.63  \\
%           & 2     & 45.87  & 52.73  & 57.76  & 60.07  & 64.61  & 67.84  & 64.98  & 67.49  & 68.91  \\
%           & 3     & 30.99  & 35.15  & 39.10  & 56.24  & 59.16  & 64.06  & 57.51  & 60.23  & 63.13  \\
%           & 4     & 29.49  & 29.67  & 28.55  & 54.84  & 57.31  & 61.37  & 54.17  & 57.17  & 60.33  \\
%           & 5     & 29.69  & 26.51  & 22.15  & 53.13  & 55.24  & 57.55  & 51.96  & 54.53  & 56.42  \\
%     \midrule
%     \multicolumn{1}{l|}{\multirow{5}[2]{*}{brightness}} & 1     & 62.16  & 61.89  & 61.65  & 70.80  & 70.45  & 69.80  & 72.22  & 72.12  & 72.07  \\
%           & 2     & 55.42  & 55.61  & 55.63  & 69.09  & 68.57  & 67.88  & 70.29  & 70.33  & 69.92  \\
%           & 3     & 51.06  & 51.15  & 51.21  & 67.15  & 67.07  & 66.54  & 68.63  & 68.69  & 68.55  \\
%           & 4     & 48.37  & 48.65  & 48.92  & 65.18  & 65.08  & 64.73  & 66.48  & 66.82  & 66.74  \\
%           & 5     & 47.11  & 47.25  & 47.46  & 63.29  & 63.25  & 62.93  & 65.20  & 65.14  & 65.26  \\
%     \midrule
%     \multicolumn{1}{l|}{\multirow{5}[2]{*}{spatter}} & 1     & 65.77  & 65.77  & 65.38  & 70.59  & 70.47  & 70.03  & 72.85  & 72.82  & 72.76  \\
%           & 2     & 52.63  & 52.91  & 51.57  & 64.02  & 62.91  & 60.68  & 69.30  & 68.38  & 66.92  \\
%           & 3     & 48.29  & 47.92  & 47.80  & 56.18  & 53.76  & 50.98  & 63.17  & 61.95  & 59.78  \\
%           & 4     & 56.52  & 56.68  & 57.01  & 61.29  & 61.25  & 61.00  & 63.82  & 62.97  & 62.10  \\
%           & 5     & 52.61  & 53.26  & 53.60  & 58.37  & 57.76  & 56.74  & 59.54  & 59.20  & 58.83  \\
%     \bottomrule
%     \end{tabular}%
% \end{table}%











% \end{document}
