# Supplementary material for: Diffusion Model Driven Test-Time Image Adaptation for Robust Skin Lesion Classification
Source: arXiv:2405.11289 source file (2024-05-18)
Supplement: Supplementary file 2 [file 0-appendix.tex]

\clearpage
\newpage

\appendix


\section{Ablation}

\subsection{Ablation on Self-Ensembling}

Since diffusion models themselves are not omnipotent, we propose a prediction fusion mechanism (Section \ref{subsec:ensemble}) to automatically choose the better candidate between an image pair, the vanilla test image, and the diffusion model's generation.
Entropy and confidence seem to be proper signals used for prediction fusion.
According to Tent~\cite{wang2021tent}, they are amazing signals indicating the potential of a prediction.
To some extent, the lower (higher) a prediction's entropy (confidence) is, the higher accuracy it would obtain.
Based on the entropy (confidence) of a prediction, we study some possibilities to utilize the image pair better.
Our exploration includes two parts, hard selection, and soft fusion,
which simply selects an image from the image pair and fuses the image pair into one new image, respectively.
The soft fusion can be operated on both pixel and logit levels.

\paragraph{Hard Selection}
Since entropy (confidence) can reflect the real accuracy of a prediction, a simple idea is to pick the image, logits of which have lower entropy (higher confidence) to make the final prediction.


\paragraph{Early Fusion}
Apart from the hard selection which selects an image from two,
we can fuse two images on the pixel level into a new one according to entropy (confidence).
We simply fuse two images, $X_1$ and $X_2$, using the weighted sum $F(a, b; f)$, where weights are from the entropy (confidence) of two images' logits, $y_1$ and $y_2$. We use a softmax operation to ensure the sum of two weights is one.

\begin{equation}
	F(a, b; f) = [a * f(X_1) + b * f(X_2)] / [f(X_1) + f(X_2)]
\end{equation}
It is worth noting that when using confidence, an image's weight is from its confidence, $conf(\cdot)$. The new image is $X_{new} = F(X_1, X_2; confidence)$. As for the entropy weight, it is from the other image's entropy, $ent(\cdot)$. The corresponding new image is $X_{new} = F(X_2, X_1; entropy)$.

\paragraph{Late Fusion}
Logits are also an excellent perspective for prediction fusion. We can take a similar strategy as the early fusion to fuse the logits, rather than image pixels.
As for confidence fusion, the new image is $y_{new} = F(y_1, y_2; confidence)$. As for the entropy fusion, the new image is $y_{new} = F(y_2, y_1; entropy)$.

As can be seen in Table~\ref{tab:ablationImageNetC2in1}, late fusion shows a better performance in all six models. Experiments have shown that the prediction fusion can effectively combine information from both the test image and the diffusion model's generation, and make a more accurate precision.

\input{tab/ablationImageNetC2in1}

\input{fig/one_out_of_two_appendix}

\paragraph{The additional evaluation of Self-Ensembling}
Figure~\ref{fig:one_out_of_two_appendix} evaluates the self-ensembling among DDA and state-of-the-art diffusion for adversarial defense (DiffPure).
It is shown that the ensembling leads to better performance for most corruption types,
and that the overall performance improvement is consistent for different image classification models.
DDA is the best on average, even DDA without self-ensembling improves on DiffPure with self-ensembling, which shows the generality of our method, since both a strong domain shift and a weak one can be covered by DDA.

\subsection{Ablation on Diffusion Models}

We investigate different choices for scaling factor $D$ and guidance scale $\boldsymbol{w}$  for latent guidance, related results of which are presented in Table~\ref{appendixTab:diffusionscalingfactor} and Table~\ref{appendixTab:diffusionrefinementrange}.
if $\boldsymbol{w}$ is too small, the guidance of the target image will not take effect. On the contrary, if $\boldsymbol{w}$ is too large, the shifting domain will bring a side effect.
The refinement range $D$ has the same effect as $\boldsymbol{w}$.
If $D$ is too small, the corruption on the target image will interfere the sampling process.
If the scaling factor $D$ is too large, the semantics information will be filtered by the low-pass filtering operation.
The results in Table~\ref{appendixTab:diffusionscalingfactor} and Table~\ref{appendixTab:diffusionrefinementrange} confirm the effect of the hyper-parameters $D$ and $\boldsymbol{w}$.

\input{tab/appendix_scalingfactor}
\input{tab/appendix_refinementrange}

\section{Tent, MEMO, BUFR, and DiffPure}


\subsection{Implementation}

Model adaptation, including Tent, MEMO, and BUFR, is sensitive to optimization hyper-parameter, especially learning rate and optimizer type. We also compare with the input adaptation Methods DiffPure~\cite{nie2022diffusion}  We introduce the hyper-parameter in this part for the four methods.

\paragraph{Tent}
\label{sec:tent_hyperparameters}
We augment the entropy loss $\mathcal{L}_{ent}$ from Tent~\cite{wang2021tent} with the additional diversity loss $\mathcal{L}_{div}$,
following the practice of SHOT~\cite{liang2020we}.
The test-time training objective is the linear combination of these two losses.
 $\mathcal{L}=\mathcal{L}_{ent} + \mathcal{L}_{div}$:
\begin{equation}
\begin{split}
    \mathcal{L}_{ent}&=-\Sigma_c p(\hat{y}_c)\log(p(\hat{y}_c) \\
    \mathcal{L}_{div}&=\kld{\hat{y}}{\frac{1}{C}\mathbf{1}_{C}} - \log(C) \\
\end{split}
\end{equation}
where $C$ is the number of classes.
$p(\hat{y}_c)$ denotes the c-th category probability in prediction $\hat{y}$.
$\mathbf{1}_{C}$ is an all-one vector with $C$ dimensions.
Therefore, $\frac{1}{C}\mathbf{1}_{C}$ indicates that every class has the same evenly distributed $\frac{1}{C}$ probabilities.
$D_{\text{KL}}$ is the notation of Kullback-Leibler divergence.

Since most recent architectures, such as ViT~\cite{dosovitskiy2021image},
do not have BatchNorm layers anymore,
we thus extend the training parameter to the whole parameter except the final classification layer.
As for ResNet-like backbones, such as ResNet-50~\cite{he2016deep},
we choose SGD as an optimizer with a learning rate $0.001$, momentum $0.9$, and weight decay $0.0001$.
As for Transformer-like backbones, such as Swin-T~\cite{liu2021swin} and ConvNeXt-T~\cite{liu2022convnet},
we choose AdamW as an optimizer with a learning rate of $0.00001$, weight decay $0.05$.
The reason behind the difference in optimizer is to follow the optimizer choice of the corresponding ImageNet training recipe.

Since the purpose of test-time adaptation is to equip the recognition model with a simple yet effective way to adapt itself,
we do not change the hyper-parameter for either single or mixed domain settings. Also, there is no prior knowledge of what test domain is before the model's deployment. We cannot choose the best hyper-parameter to accompany the test-time sampling policy, batch size, \etc.
We observe that model adaptation is highly sensitive to the choice of optimization hyper-parameters.
The ablation of learning rate and optimizer type could be found in Figure~\ref{fig:lr_sgd_adamw_single} and Figure~\ref{fig:lr_sgd_adamw_multi}.

\input{fig/lr_sgd_adamw}

\paragraph{MEMO}
Following the official repository of MEMO~\cite{zhang2021memo}, we choose SGD as the optimizer with a learning rate of $0.00025$. We have also explored the optimizer type and lr for different models and experiments show that the official setting is the best.


\paragraph{BUFR}
Since the  official repository of BUFR~\cite{eastwood2021source} did not conduct the experiments on ImageNet-C with ResNet-50, we choose SGD as the optimizer with a learning rate of $0.001$. The epochs per block is 3. Trained with ordered data, the average accuracy for BUFR is 2.8\% / 17.9\% accuracy when batch size is 1 / 64. When the class order is fixed, and the batch size is 64, BUFR achieved 4.2\% / 3.4\% with mixed/unmixed types. When the class order is shuffled, and the batch size is 64, BUFR achieved 4.3\% / 8.3\% with mixed/unmixed types. The results demonstrate that the limited, ordered, or mixed data does affect the training process and the classification accuracy.

\paragraph{DiffPure}
DiffPure~\cite{nie2022diffusion} simply adds a given amount of noise and then reverses to $t = 0$.
Following the official repository of DiffPure, we set the hyperparameter $t=150$


\subsection{Results}

\paragraph{Benchmark Evaluation (Independent Adaptation): Tent and DDA}
Table~\ref{tab:mCEImageNetCsingle} depicts the performance of Tent\cite{wang2021tent} and our DDA in 8 models.
The first models, ResNet50, Swin-T, and ConvNeXt-T, are already mentioned in Sec~\ref{sec:models}.
Here we additionally provide more experiments in much larger models, Swin transformer Base (Swin-B) and ConvNeXt Base (ConvNeXt-B).
It is worth noting that we provide two versions of base models: 1) trained with ImageNet-1K only (denote as Swin-B and ConvNeXt-B), 2) pretrained with ImageNet-21K first and then finetuned with ImageNet-1K (denote as Swin-B* and ConvNeXt-B*).
When the batch size equals one, DDA can beat Tent easily according to its advantage in tackling insufficient sampling.
When the categories of test images are not shuffled, DDA still has much better performance,
even with the larger state-of-the-art architectures.

\input{tab/mCEImageNetCsingle}

\input{tab/appendix_mCEImageNetCmulti}
\paragraph{Challenge Exploration (Joint Adaptation): Offline Tent}
In Table~\ref{tab:appendix_mCEImageNetCmulti}, we provide a more detailed comparison between episodic, online, and offline model adaptation performance.
In the first group of rows, we evaluate the episodic setting, in which adaptation and prediction are independent across inputs.
In particular, the episodic source-only, MEMO, DiffPure, and DDA methods do not depend on any data except for each input in isolation.
In the second group of rows we evaluate model adaptation by Tent in the online setting, in which adaptation and prediction are done per batch, and adaptation updates persist across batches.
(This is the setting reported in Table~\ref{tab:mCEImageNetCmulti} of the main paper, as it is the recommended setting for Tent.)
In the third group of rows, we evaluate model adaptation by Tent in the offline setting, in which the method first adapts to the entire test set, and then makes predictions for each input.
In this setting, Tent first learns from all of the data but then makes predictions with a single model that cannot specifically adapt to each batch.
Whether online or offline, Tent is sensitive to the order of the data, and fails when data arrive one by one (with a batch size of one) or when classes are not mixed by shuffling.

\input{fig/multi_domain_batch}
\paragraph{Challenge Exploration (Joint Adaptation): fixed and shuffled class order}
As shown in Figure~\ref{fig:shuffle_batchsize_multi_shuffle} and Figure~\ref{fig:shuffle_batchsize_multi_noshuffle},
the shuffled class order is essential to Tent, especially for models with low capacity.
Even for big models, the potential of Tent as the batch size increases is suppressed largely.

\section{More datasets}

\paragraph{ImageNet-W}

\input{fig/appendix_ImageNetW}

ImageNet-W~\cite{li2022whacamole} is an evaluation set based on ImageNet for the watermark. The authors found that the watermark as a shortcut affects nearly every modern vision model. In our experimental settings, the watermark can be regarded as a common corruption by human activities, as a supplement dataset of the unexpected corruptions, ImageNet-C (IN-C)~\cite{hendrycks2019robustness} and ImageNet-$\overline{\text{C}}$ (IN-$\bar{\text{C}}$)~\cite{mintun2021interaction}.
Figure~\ref{fig:appendix_imagenetw} shows that DDA can effectively remove the watermark to avoid shortcut reliance.
Our experiments, conducted on ImagenNet-W using ResNet-50, showed that DDA achieved 58.3\% accuracy, a significant improvement over the baseline accuracy of 47.4\%. Both the visualizations and model performance demonstrate that DDA can enhance the robustness of the model against watermark corruption.

\paragraph{ImageNet-R}

ImageNet-R~\cite{hendrycks2021many} is an evaluation set based on ImageNet for rendition, containing cartoons, embroidery, graphics, paintings, sketches, tattoos, toys, and so on.
Our qualitative experiments in Figure~\ref{fig:appendix_imagenetr} depict the performance of DDA on rendition to real images. Although the adapted images still reserve the original background, real-world characteristics have been added to the main part of the picture. DDA easily concentrates on the core domain shift in the renditions, especially for the gap between the 2D and 3D features.

\input{fig/appendix_ImageNetR}


\section{Visualization}

\paragraph{Progressive generation on ImageNet-C and ImageNet}

\input{fig/appendix_timestep}

Figure~\ref{appendixFig:timestep} illustrates how diffusion models denoise and reconstruct the given corrupted images.
Here we take elastic transformation, glass blur, and shot noise as the representative corruption for the digital artifact, natural blur, and common noise.
We observe that diffusion models are able to clean up the \say{local}, high-frequency noises, \ie Gaussian noise, pixelate, etc.
As for \say{global}, low-frequency corruption, \ie fog, snow, \etc, diffusion models failed to recover the original version.
One reason behind this phenomenon could be these low-frequency corrupted images are treated as natural samples during ImageNet training.
In other words, the diffusion model is trained on ImageNet, which may cover several augmentations including these low-frequency corruptions.

\input{fig/timestep_origin}

Figure~\ref{fig:timestep_origin} visualizes the procedure given the original ImageNet validation images.
We observe that images after diffusion are almost the same as the original ones.
In general, the reconstructions from diffusion models look similar to the original ImageNet validation images, which indicates the effectiveness of the leveraged generative models.
It is worth noting the comparison between the output and the original in the second row, peacock. Diffusion models hallucinate more details on the left that do not exist in the original input image.


\paragraph{Qualitative results on success and failure Cases}

\input{fig/corruption_positive}
\input{fig/corruption_negative}

We visualize success and failure cases across corruptions on ImageNet-C as shown in Figure~\ref{fig:corruption_positive} and Figure~\ref{fig:corruption_negative}.
DDA forces the model to preserve the global structural information to avoid semantic drift,
leading to a drawback that it may fail to adapt images from certain domains.
While DDA performs well when projecting most high-frequency/local corruptions (\eg, Gaussian noise, impulse noise, jpeg encoding, \ldots),
it fails for a few low-frequency/global corruptions (\eg, frost, fog, brightness adjustment, \ldots).
However, our self-ensembling scheme effectively detects these cases to avoid significant drops in accuracy.
