# Supplementary material for: Diffusion Model Driven Test-Time Image Adaptation for Robust Skin Lesion Classification
Source: arXiv:2405.11289 source file (2024-05-18)
Supplement: Supplementary file 3 [file appendix_ImageNetR.tex]

\begin{figure*}[htbp]
    \begin{center}
    	\adjustbox{max width=\linewidth}{
            \begin{tabular}{c c c c c c c c c}
                & \resizebox{!}{0.6in}{cartoon} & \resizebox{!}{0.7in}{misc} & \resizebox{!}{0.7in}{painting} & \resizebox{!}{0.7in}{sketch} & \resizebox{!}{0.7in}{videogame} & \resizebox{!}{0.7in}{embroidery} & \resizebox{!}{0.6in}{tattoo} & \resizebox{!}{0.7in}{graphic} \\
                & & & & & & & & \\
                \resizebox{0.75in}{!}{\rotatebox{90}{ImageNet-R}} &
                \includegraphics[width=\linewidth]{imagenet-r/cartoon_origin} &
                \includegraphics[width=\linewidth]{imagenet-r/misc_origin} &
                \includegraphics[width=\linewidth]{imagenet-r/painting_origin} &
                \includegraphics[width=\linewidth]{imagenet-r/sketch_origin} &
                \includegraphics[width=\linewidth]{imagenet-r/videogame_origin} &
                \includegraphics[width=\linewidth]{imagenet-r/embroidery_origin} &
                \includegraphics[width=\linewidth]{imagenet-r/tattoo_origin} &
                \includegraphics[width=\linewidth]{imagenet-r/graphic_origin} \\
                
                & & & & & & & & \\
                \resizebox{0.75in}{!}{\rotatebox{90}{DDA Output}} &
                \includegraphics[width=\linewidth]{imagenet-r/cartoon_dda} &
                \includegraphics[width=\linewidth]{imagenet-r/misc_dda} &
                \includegraphics[width=\linewidth]{imagenet-r/painting_dda} &
                \includegraphics[width=\linewidth]{imagenet-r/sketch_dda} &
                \includegraphics[width=\linewidth]{imagenet-r/videogame_dda} &
                \includegraphics[width=\linewidth]{imagenet-r/embroidery_dda} &
                \includegraphics[width=\linewidth]{imagenet-r/tattoo_dda} &
                \includegraphics[width=\linewidth]{imagenet-r/graphic_dda} \\
                
                
            \end{tabular}
    	}

	\end{center}
% 	\vspace{2mm}
% 	\vspace{-3mm}
	\caption{Visualization of generated images with DDA on ImageNet-R.}
	\label{fig:appendix_imagenetr}
\end{figure*}
