# Supplementary material for: Diffusion Model Driven Test-Time Image Adaptation for Robust Skin Lesion Classification
Source: arXiv:2405.11289 source file (2024-05-18)
Supplement: Supplementary file 4 [file appendix_ImageNetW.tex]

\begin{figure*}[htbp]
    \begin{center}
    	\adjustbox{max width=\linewidth}{
            \begin{tabular}{c c c c c c c c c}
               
                \resizebox{0.75in}{!}{\rotatebox{90}{ImageNet-W}} &
                \includegraphics[width=\linewidth]{imagenet-w/ILSVRC2012_val_00005567} &
                \includegraphics[width=\linewidth]{imagenet-w/ILSVRC2012_val_00008028} &
                \includegraphics[width=\linewidth]{imagenet-w/ILSVRC2012_val_00046547} &
                \includegraphics[width=\linewidth]{imagenet-w/ILSVRC2012_val_00028159} &
                \includegraphics[width=\linewidth]{imagenet-w/ILSVRC2012_val_00030818} &
                \includegraphics[width=\linewidth]{imagenet-w/ILSVRC2012_val_00031333} &
                \includegraphics[width=\linewidth]{imagenet-w/ILSVRC2012_val_00024665} &
                \includegraphics[width=\linewidth]{imagenet-w/ILSVRC2012_val_00045741} \\
                
                
                & & & & & & & \\
                \resizebox{0.75in}{!}{\rotatebox{90}{DDA Output}} &
                \includegraphics[width=\linewidth]{imagenet-w-dda/ILSVRC2012_val_00005567} &
                \includegraphics[width=\linewidth]{imagenet-w-dda/ILSVRC2012_val_00008028} &
                \includegraphics[width=\linewidth]{imagenet-w-dda/ILSVRC2012_val_00046547} &
                \includegraphics[width=\linewidth]{imagenet-w-dda/ILSVRC2012_val_00028159} &
                \includegraphics[width=\linewidth]{imagenet-w-dda/ILSVRC2012_val_00030818} &
                \includegraphics[width=\linewidth]{imagenet-w-dda/ILSVRC2012_val_00031333} &
                \includegraphics[width=\linewidth]{imagenet-w-dda/ILSVRC2012_val_00024665} &
                \includegraphics[width=\linewidth]{imagenet-w-dda/ILSVRC2012_val_00045741} \\
                 
                
                
            \end{tabular}
    	}

	\end{center}
% 	\vspace{2mm}
% 	\vspace{-3mm}
	\caption{Visualization of generated images with DDA output on ImageNet-W.}
	\label{fig:appendix_imagenetw}
\end{figure*}
