# Supplementary material for: Diffusion Model Driven Test-Time Image Adaptation for Robust Skin Lesion Classification
Source: arXiv:2405.11289 source file (2024-05-18)
Supplement: Supplementary file 5 [file appendix_timestep.tex]

\begin{figure*}[ht]
    \begin{center}
    	\adjustbox{max width=0.78\linewidth}{
            \begin{tabular}{c c c c c c c c}
                \resizebox{!}{0.7in}{corrupted} & \resizebox{!}{0.7in}{input} & \resizebox{!}{0.7in}{20\%} & \resizebox{!}{0.7in}{40\%} & \resizebox{!}{0.7in}{60\%} & \resizebox{!}{0.7in}{80\%} & \resizebox{!}{0.6in}{output} & \resizebox{!}{0.7in}{original} \\
                & & & & & & & \\
                & & & & & & & \\
                \includegraphics[width=\linewidth]{imagenet-c/elastic_transform/5/n01531178/ILSVRC2012_val_00005567} &
                \includegraphics[width=\linewidth]{timestep/elastic_transform_5/ILSVRC2012_val_00005567_49} &
                \includegraphics[width=\linewidth]{timestep/elastic_transform_5/ILSVRC2012_val_00005567_40} &
                \includegraphics[width=\linewidth]{timestep/elastic_transform_5/ILSVRC2012_val_00005567_30} &
                \includegraphics[width=\linewidth]{timestep/elastic_transform_5/ILSVRC2012_val_00005567_20} &
                \includegraphics[width=\linewidth]{timestep/elastic_transform_5/ILSVRC2012_val_00005567_10} &
                \includegraphics[width=\linewidth]{timestep/elastic_transform_5/ILSVRC2012_val_00005567_0} &
                \includegraphics[width=\linewidth]{timestep/ILSVRC2012_val_00005567_r256c224} \\
                & & & & & & & \\
                \includegraphics[width=\linewidth]{imagenet-c/elastic_transform/5/n01871265/ILSVRC2012_val_00046757} &
                \includegraphics[width=\linewidth]{timestep/elastic_transform_5/ILSVRC2012_val_00046757_49} &
                \includegraphics[width=\linewidth]{timestep/elastic_transform_5/ILSVRC2012_val_00046757_40} &
                \includegraphics[width=\linewidth]{timestep/elastic_transform_5/ILSVRC2012_val_00046757_30} &
                \includegraphics[width=\linewidth]{timestep/elastic_transform_5/ILSVRC2012_val_00046757_20} &
                \includegraphics[width=\linewidth]{timestep/elastic_transform_5/ILSVRC2012_val_00046757_10} &
                \includegraphics[width=\linewidth]{timestep/elastic_transform_5/ILSVRC2012_val_00046757_0} &
                \includegraphics[width=\linewidth]{ablation/origin/ILSVRC2012_val_00046757} \\
                & & & & & & & \\
                \includegraphics[width=\linewidth]{imagenet-c/elastic_transform/5/n01806143/ILSVRC2012_val_00028159} &
                \includegraphics[width=\linewidth]{timestep/elastic_transform_5/ILSVRC2012_val_00028159_49} &
                \includegraphics[width=\linewidth]{timestep/elastic_transform_5/ILSVRC2012_val_00028159_40} &
                \includegraphics[width=\linewidth]{timestep/elastic_transform_5/ILSVRC2012_val_00028159_30} &
                \includegraphics[width=\linewidth]{timestep/elastic_transform_5/ILSVRC2012_val_00028159_20} &
                \includegraphics[width=\linewidth]{timestep/elastic_transform_5/ILSVRC2012_val_00028159_10} &
                \includegraphics[width=\linewidth]{timestep/elastic_transform_5/ILSVRC2012_val_00028159_0} &
                \includegraphics[width=\linewidth]{timestep/ILSVRC2012_val_00028159_r256c224} \\
                & & & & & & & \\
                \includegraphics[width=\linewidth]{imagenet-c/elastic_transform/5/n02093256/ILSVRC2012_val_00046547} &
                \includegraphics[width=\linewidth]{timestep/elastic_transform_5/ILSVRC2012_val_00046547_49} &
                \includegraphics[width=\linewidth]{timestep/elastic_transform_5/ILSVRC2012_val_00046547_40} &
                \includegraphics[width=\linewidth]{timestep/elastic_transform_5/ILSVRC2012_val_00046547_30} &
                \includegraphics[width=\linewidth]{timestep/elastic_transform_5/ILSVRC2012_val_00046547_20} &
                \includegraphics[width=\linewidth]{timestep/elastic_transform_5/ILSVRC2012_val_00046547_10} &
                \includegraphics[width=\linewidth]{timestep/elastic_transform_5/ILSVRC2012_val_00046547_0} &
                \includegraphics[width=\linewidth]{timestep/ILSVRC2012_val_00046547_r256c224} \\
                & & & & & & & \\
                \midrule[3mm]
                & & & & & & & \\
                \includegraphics[width=\linewidth]{imagenet-c/glass_blur/5/n01531178/ILSVRC2012_val_00005567} &
                \includegraphics[width=\linewidth]{timestep/glass_blur_5/ILSVRC2012_val_00005567_49} &
                \includegraphics[width=\linewidth]{timestep/glass_blur_5/ILSVRC2012_val_00005567_40} &
                \includegraphics[width=\linewidth]{timestep/glass_blur_5/ILSVRC2012_val_00005567_30} &
                \includegraphics[width=\linewidth]{timestep/glass_blur_5/ILSVRC2012_val_00005567_20} &
                \includegraphics[width=\linewidth]{timestep/glass_blur_5/ILSVRC2012_val_00005567_10} &
                \includegraphics[width=\linewidth]{timestep/glass_blur_5/ILSVRC2012_val_00005567_0} &
                \includegraphics[width=\linewidth]{timestep/ILSVRC2012_val_00005567_r256c224} \\
                & & & & & & & \\
                \includegraphics[width=\linewidth]{imagenet-c/glass_blur/5/n01871265/ILSVRC2012_val_00046757} &
                \includegraphics[width=\linewidth]{timestep/glass_blur_5/ILSVRC2012_val_00046757_49} &
                \includegraphics[width=\linewidth]{timestep/glass_blur_5/ILSVRC2012_val_00046757_40} &
                \includegraphics[width=\linewidth]{timestep/glass_blur_5/ILSVRC2012_val_00046757_30} &
                \includegraphics[width=\linewidth]{timestep/glass_blur_5/ILSVRC2012_val_00046757_20} &
                \includegraphics[width=\linewidth]{timestep/glass_blur_5/ILSVRC2012_val_00046757_10} &
                \includegraphics[width=\linewidth]{timestep/glass_blur_5/ILSVRC2012_val_00046757_0} &
                \includegraphics[width=\linewidth]{ablation/origin/ILSVRC2012_val_00046757} \\
                & & & & & & & \\
                \includegraphics[width=\linewidth]{imagenet-c/glass_blur/5/n01806143/ILSVRC2012_val_00028159} &
                \includegraphics[width=\linewidth]{timestep/glass_blur_5/ILSVRC2012_val_00028159_49} &
                \includegraphics[width=\linewidth]{timestep/glass_blur_5/ILSVRC2012_val_00028159_40} &
                \includegraphics[width=\linewidth]{timestep/glass_blur_5/ILSVRC2012_val_00028159_30} &
                \includegraphics[width=\linewidth]{timestep/glass_blur_5/ILSVRC2012_val_00028159_20} &
                \includegraphics[width=\linewidth]{timestep/glass_blur_5/ILSVRC2012_val_00028159_10} &
                \includegraphics[width=\linewidth]{timestep/glass_blur_5/ILSVRC2012_val_00028159_0} &
                \includegraphics[width=\linewidth]{timestep/ILSVRC2012_val_00028159_r256c224} \\
                & & & & & & & \\
                \includegraphics[width=\linewidth]{imagenet-c/glass_blur/5/n02093256/ILSVRC2012_val_00046547} &
                \includegraphics[width=\linewidth]{timestep/glass_blur_5/ILSVRC2012_val_00046547_49} &
                \includegraphics[width=\linewidth]{timestep/glass_blur_5/ILSVRC2012_val_00046547_40} &
                \includegraphics[width=\linewidth]{timestep/glass_blur_5/ILSVRC2012_val_00046547_30} &
                \includegraphics[width=\linewidth]{timestep/glass_blur_5/ILSVRC2012_val_00046547_20} &
                \includegraphics[width=\linewidth]{timestep/glass_blur_5/ILSVRC2012_val_00046547_10} &
                \includegraphics[width=\linewidth]{timestep/glass_blur_5/ILSVRC2012_val_00046547_0} &
                \includegraphics[width=\linewidth]{timestep/ILSVRC2012_val_00046547_r256c224} \\
                & & & & & & & \\
                \midrule[3mm]
                & & & & & & & \\
                \includegraphics[width=\linewidth]{imagenet-c/shot_noise/5/n01531178/ILSVRC2012_val_00005567} &
                \includegraphics[width=\linewidth]{timestep/shot_noise_5/ILSVRC2012_val_00005567_49} &
                \includegraphics[width=\linewidth]{timestep/shot_noise_5/ILSVRC2012_val_00005567_40} &
                \includegraphics[width=\linewidth]{timestep/shot_noise_5/ILSVRC2012_val_00005567_30} &
                \includegraphics[width=\linewidth]{timestep/shot_noise_5/ILSVRC2012_val_00005567_20} &
                \includegraphics[width=\linewidth]{timestep/shot_noise_5/ILSVRC2012_val_00005567_10} &
                \includegraphics[width=\linewidth]{timestep/shot_noise_5/ILSVRC2012_val_00005567_0} &
                \includegraphics[width=\linewidth]{timestep/ILSVRC2012_val_00005567_r256c224} \\
                & & & & & & & \\
                \includegraphics[width=\linewidth]{imagenet-c/shot_noise/5/n01871265/ILSVRC2012_val_00046757} &
                \includegraphics[width=\linewidth]{timestep/shot_noise_5/ILSVRC2012_val_00046757_49} &
                \includegraphics[width=\linewidth]{timestep/shot_noise_5/ILSVRC2012_val_00046757_40} &
                \includegraphics[width=\linewidth]{timestep/shot_noise_5/ILSVRC2012_val_00046757_30} &
                \includegraphics[width=\linewidth]{timestep/shot_noise_5/ILSVRC2012_val_00046757_20} &
                \includegraphics[width=\linewidth]{timestep/shot_noise_5/ILSVRC2012_val_00046757_10} &
                \includegraphics[width=\linewidth]{timestep/shot_noise_5/ILSVRC2012_val_00046757_0} &
                \includegraphics[width=\linewidth]{ablation/origin/ILSVRC2012_val_00046757} \\
                & & & & & & & \\
                \includegraphics[width=\linewidth]{imagenet-c/shot_noise/5/n01806143/ILSVRC2012_val_00028159} &
                \includegraphics[width=\linewidth]{timestep/shot_noise_5/ILSVRC2012_val_00028159_49} &
                \includegraphics[width=\linewidth]{timestep/shot_noise_5/ILSVRC2012_val_00028159_40} &
                \includegraphics[width=\linewidth]{timestep/shot_noise_5/ILSVRC2012_val_00028159_30} &
                \includegraphics[width=\linewidth]{timestep/shot_noise_5/ILSVRC2012_val_00028159_20} &
                \includegraphics[width=\linewidth]{timestep/shot_noise_5/ILSVRC2012_val_00028159_10} &
                \includegraphics[width=\linewidth]{timestep/shot_noise_5/ILSVRC2012_val_00028159_0} &
                \includegraphics[width=\linewidth]{timestep/ILSVRC2012_val_00028159_r256c224} \\
                & & & & & & & \\
                \includegraphics[width=\linewidth]{imagenet-c/shot_noise/5/n02093256/ILSVRC2012_val_00046547} &
                \includegraphics[width=\linewidth]{timestep/shot_noise_5/ILSVRC2012_val_00046547_49} &
                \includegraphics[width=\linewidth]{timestep/shot_noise_5/ILSVRC2012_val_00046547_40} &
                \includegraphics[width=\linewidth]{timestep/shot_noise_5/ILSVRC2012_val_00046547_30} &
                \includegraphics[width=\linewidth]{timestep/shot_noise_5/ILSVRC2012_val_00046547_20} &
                \includegraphics[width=\linewidth]{timestep/shot_noise_5/ILSVRC2012_val_00046547_10} &
                \includegraphics[width=\linewidth]{timestep/shot_noise_5/ILSVRC2012_val_00046547_0} &
                \includegraphics[width=\linewidth]{timestep/ILSVRC2012_val_00046547_r256c224} \\
            \end{tabular}
    	}

	\end{center}
% 	\vspace{2mm}
% 	\vspace{-3mm}
	\caption{Visualization of generated images with diffusion models, given highest severity corrupted images during the test time.}
	\label{appendixFig:timestep}
\end{figure*}
