# Supplementary material for: Diffusion Model Driven Test-Time Image Adaptation for Robust Skin Lesion Classification
Source: arXiv:2405.11289 source file (2024-05-18)
Supplement: Supplementary file 6 [file one_out_of_two_appendix.tex]

\begin{figure*}[t]
\vspace{-5pt}
\begin{center}
\adjustbox{max width=0.9\linewidth}{
    % \begin{tabular}{c c}
    %     \resizebox{!}{0.2in}{\small (a) RedNet-26} &
    %     \resizebox{!}{0.2in}{\small (b) ResNet-50} \\
    %     & \\
    %     % & \\
    %     \includegraphics[width=\linewidth]{one_out_of_two/selection_RedNet26_top1} &
    %     \includegraphics[width=\linewidth]{one_out_of_two/selection_ResNet50_top1} \\
    %     \resizebox{!}{0.2in}{\small (c) Swin-Tiny} &
    %     \resizebox{!}{0.2in}{\small (d) ConvNeXt-Tiny} \\
    %     & \\
    %     % & \\
    %     \includegraphics[width=\linewidth]{one_out_of_two/selection_Swin-T_top1} &
    %     \includegraphics[width=\linewidth]{one_out_of_two/selection_ConvNeXt-T_top1} \\
    % \end{tabular}

    % https://latexdraw.com/how-to-annotate-an-image-in-latex/
    \begin{tabular}{c}
      \begin{tikzpicture}
        % Include the image in a node
        \node [
          above right,
          inner sep=0
        ] (image) at (0,0) {\includegraphics[width=\textwidth]{one_out_of_two/version1/5bar_gradient_selection_ResNet50_top1}};

        % Create scope with normalized axes
        \begin{scope}[
        x={($0.1*(image.south east)$)},
        y={($0.1*(image.north west)$)}]

        % Labels
        \node[above,black] at (4.5,5.1) {\normalsize (a) ResNet-50};

        \end{scope}
      \end{tikzpicture} \\
      \begin{tikzpicture}
        % Include the image in a node
        \node [
          above right,
          inner sep=0
        ] (image) at (0,0) {\includegraphics[width=\textwidth]{one_out_of_two/version1/5bar_gradient_selection_Swin-T_top1.pdf}};

        % Create scope with normalized axes
        \begin{scope}[
        x={($0.1*(image.south east)$)},
        y={($0.1*(image.north west)$)}]

        % Labels
        \node[above,black] at (4.5,5.1) {\normalsize (b) Swin-Tiny};

        \end{scope}
      \end{tikzpicture} \\
      \begin{tikzpicture}
        % Include the image in a node
        \node [
          above right,
          inner sep=0
        ] (image) at (0,0) {\includegraphics[width=\textwidth]{one_out_of_two/version1/5bar_gradient_selection_ConvNeXt-T_top1}};

        % Create scope with normalized axes
        \begin{scope}[
        x={($0.1*(image.south east)$)},
        y={($0.1*(image.north west)$)}]

        % Labels
        \node[above,black] at (4.5,5.1) {\normalsize (c) ConvNeXt-Tiny};

        \end{scope}
      \end{tikzpicture} \\
  \end{tabular}
}
\end{center}
\vspace{-4mm}
\caption{%
    \textbf{Self-Ensembling reliably improves robustness across corruption types.}
    We evaluate the self-ensembling among DDA and state-of-the-art diffusion for adversarial defense (DiffPure). Self-Ensembling prevents catastrophic drops (on fog or contrast, for example) and improves the performance on DDA and DiffPure. DDA is the best on average, even DDA without self-ensembling improves on DiffPure with self-ensembling.
}
% Classification accuracy on different corruption types of ImageNet-C at maximum severity (level 5).
% Higher is better.
% ``Source-only'' denotes the source-only test where the corrupted image is fed into the image classifier without adaptation.
% ``Diffusion'' denotes DDA without self-ensembling.
% ``DDA'' denotes the final result of our approach with self-ensembling.
% We observe that DDA brings additional improvement on the top of diffusion.

% \vspace{-3mm}
\label{fig:one_out_of_two_appendix}
\end{figure*}
