# Supplementary material for: Diffusion Model Driven Test-Time Image Adaptation for Robust Skin Lesion Classification
Source: arXiv:2405.11289 source file (2024-05-18)
Supplement: Supplementary file 7 [file appendix_mCEImageNetCmulti.tex]

\begin{table}
  \caption{%
    \textbf{DDA is reliably more robust when the target data is limited, ordered, or mixed.}
    Deployment may supply target data in various ways.
    To explore these regimes, we vary batch size and whether or not the data is ordered by class or mixed across corruption types.
    We compare episodic adaptation by input updates with DDA (ours) and by model updates with MEMO along with cumulative adaptation by Tent.
    DDA and MEMO are invariant to these differences.
    However, Tent is highly sensitive to batch size and order, and fails on ordered classes and mixed types.
  }
  \label{tab:appendix_mCEImageNetCmulti}
  \begin{center}
  \adjustbox{max width=\linewidth}{
  % \Huge
  \huge
  % \large
  \renewcommand\arraystretch{1.2}
    \begin{tabular}{c|cc|c|c|cc}
      \toprule
      Method &
      \pbox{3em}{Mixed \\ Classes} &
      \pbox{6em}{Mixed \\ Types} &
      Batch Size &
      % RedNet-26 &
      ResNet-50 &
      Swin-T &
      ConvNeXt-T \\
      % Swin-B &
      % ConvNeXt-B \\
      % \midrule
      % \xmark & \xmark & 97.1 & 97.8 & 99.8 & 99.9 & 99.7 & 97.0 \\
      % \xmark & \cmark & 95.9 & 98.4 & 99.8 & 99.7 & 99.6 & 97.1 \\
      % \cmark & \xmark & 96.6 & 97.0 & 99.9 & 99.8 & 99.6 & 91.5 \\
      % \cmark & \cmark & 95.2 & 97.7 & 99.7 & 99.7 & 99.6 & 88.8 \\
      % \midrule
      % \multicolumn{2}{c|}{source-only test} & 85.0 & 81.3 & 66.9 & 60.7 & 59.0 & 54.4 \\
      % \multicolumn{2}{c|}{MEMO~\cite{zhang2021memo}} & & & & & & \\
      % % \multicolumn{2}{c|}{BUFR~\cite{eastwood2021source}} & & & & & & \\
      % \rowcolor{lightgray}
      % \multicolumn{2}{c|}{DDA (ours)} & \textbf{75.1} & \textbf{72.8} & \textbf{63.3} & \textbf{58.9} & \textbf{58.0} & \textbf{53.9} \\
      \midrule
      Source-Only & \multicolumn{2}{c|}{\multirow{4}{*}{N/A}} & \multirow{4}{*}{N/A} 
      % & 15.0 
      & 18.7 & 33.1 & 39.3 \\ %& 41.0 & 45.6 \\
      MEMO~\cite{zhang2021memo} & & & 
      % & 20.6 
      & 24.7 & 29.5 & 37.8 \\ %& 37.0 & 45.8 \\
      DiffPure~\cite{nie2022diffusion} & & &  
      & 16.8 & 24.8 & 28.8 \\
      \rowcolor{lightgray}
      DDA (ours) & & & 
      % & {\bf 25.0} 
      & {\bf 29.7} & {\bf 40.0} & {\bf 44.2} \\ %& 42.0 & 46.1 \\
      \midrule
      \multirow{4}{*}{Tent (Online)} & \xmark & \xmark & 1 / 64 
      % & 0.8  / 0.2  
      & 0.1  / 0.4  & 2.8  / 2.3  & 10.5  / 9.6 \\
      & \xmark & \cmark & 1 / 64 
      % & 0.8  / 0.3  
      & 0.1  / 0.3  & 8.0  / 2.2  & 18.8  / 6.5 \\
      & \cmark & \xmark & 1 / 64 
      % & 0.8  / \bf{7.7}  
      & 0.1  / \bf{22.6}  & 3.0  / \bf{41.0}  & 11.0  / \bf{50.1} \\
      & \cmark & \cmark & 1 / 64 
      % & 0.8  / 3.4  
      & 0.1  / 6.5  & 8.5  / 36.9  & 18.9  / 47.4  \\ %& 0.4 & 11.2 \\
      \midrule
      \multirow{4}{*}{Tent (Offline)} & \xmark & \xmark & 1 / 64 
      % & 2.9 / 0.2 
      & 2.2 / 0.4 & 0.2 / 0.2 & 0.1 / 1.4 \\ %& 0.3 & 3.0 \\
      & \xmark & \cmark & 1 / 64 
      % & 4.1 / 0.4 
      & 1.6 / 0.5 & 0.2 / 0.5 & 0.3 / 0.5 \\ %& 0.4 & 2.9 \\
      & \cmark & \xmark & 1 / 64 
      % & 3.4 / 1.9 
      & 3.0 / {\bf 7.6} & 0.1 / 43.3 & 0.2 / 48.8 \\ %& 0.4 & 8.5 \\
      & \cmark & \cmark & 1 / 64 
      % & {\bf 4.8} / 1.6 
      & 2.3 / 3.9 & 0.3 / {\bf 44.1} & 0.3 / {\bf 51.9} \\ %& 0.4 & 11.2 \\
      \midrule
      % \midrule
      % \multirow{2}{*}{\xmark} & \multirow{2}{*}{\xmark} & 1 & 97.1 & 97.8 & 99.8 & 99.9 & 99.7 & 97.0 \\
      % & & 64 & 99.8 & 99.6 & 99.8 & 98.6 & 99.8 & 99.0\\
      % \midrule
      % \multirow{2}{*}{\xmark} & \multirow{2}{*}{\cmark} & 1 & 95.9 & 98.4 & 99.8 & 99.7 & 99.6 & 97.1 \\
      %  & & 64 & 99.6 & 99.5 & 99.5 & 98.4 & 99.8 & 98.9 \\
      % \midrule
      % \multirow{2}{*}{\cmark} & \multirow{2}{*}{\xmark} & 1 & 96.6 & 97.0 & 99.9 & 99.8 & 99.6 & 91.5\\
      %  & & 64 & 98.1 & 92.4 & 56.7 & 51.2 & 49.0 & 46.7\\
      % \midrule
      % \multirow{2}{*}{\cmark} & \multirow{2}{*}{\cmark} & 1 & 95.2 & 97.7 & 99.7 & 99.7 & 99.6 &88.8\\
      %  & & 64 & 98.4 & 96.1 & 55.9 & 48.1 & 48.5 & 43.2\\
      % \midrule
      % \multicolumn{2}{c|}{source} & \multirow{2}{*}{$\forall$} & 85.0 & 81.3 & 66.9 & 60.7 & 59.0 & 54.4\\
      % \multicolumn{2}{c|}{ours} & & 75.1 & 72.8 & 63.3 & 58.9 & 58.0 & 53.9\\
      \bottomrule
  \end{tabular}}
  \end{center}
\end{table}
