# Supplementary material for: Diffusion Model Driven Test-Time Image Adaptation for Robust Skin Lesion Classification
Source: arXiv:2405.11289 source file (2024-05-18)
Supplement: Supplementary file 8 [file appendix_refinementrange.tex]

\begin{table}[t]
  \caption{
	\textbf{Ablation on choices of refinement range $\boldsymbol{w}$ with fixed $D$.} 
	Our default hyper-parameter is in the shadow row.
	The empirical results confirm the choice of hyper-parameters in DDA.
  }
  \label{appendixTab:diffusionrefinementrange}
  \begin{center}
   		\adjustbox{max width=\linewidth}{
   			\renewcommand\arraystretch{1.15}
   			\begin{tabular}{ll|ccc}
   				& $D=4$
   				% & RedNet-26
   				& ResNet-50
   				& Swin-T
   				& ConvNeXt-T
   				\\
   				\midrule
   				% \multirow{3}{*}{(a) trans}
   				& 3
   				% & 33.2     
                    & 38.0     & 42.3  & 44.9
   				\\
   				\rowcolor{lightgray} (a) elastic transformation & 6
   				% & 34.3     
                    & 32.3     & 38.9  & 41.2
   				\\
   				& 9
   				% & 33.9     
                    & 27.8     & 35.2  & 37.9
   				\\
   				\midrule
   				% \multirow{3}{*}{(b) blur}
   				& 3
   				% & 16.1     
                    & 17.9     & 24.7  & 28.7
   				\\
   				\rowcolor{lightgray} (b) glass blur & 6
   				% & 14.5     
                    & 12.0     & 17.6  & 19.9
   				\\
   				& 9
   				% & 13.4     
                    & 9.2      & 13.4  & 15.2
   				\\
   				\midrule
   				% \multirow{3}{*}{(c) noise}
   				& 3
   				% & 24.8     
                    & 48.2     & 50.5  & 54.1
   				\\
   				\rowcolor{lightgray} (c) shot noise & 6
   				% & 36.4     
                    & 48.7     & 53.2  & 57.3   
   				\\
   				& 9
   				% & 36.4     
                    & 40.7     & 49.1  & 54.4
   				\\
   				\bottomrule
   			\end{tabular}
   		}
    \end{center}
\end{table}

% \begin{table}[t]
%   \caption{
% 	\textbf{Ablation on choices of refinement range $M$ with fixed $D$.} 
% 	Our default hyper-parameter is in the shadow row.
% 	The empirical results confirm the choice of hyper-parameters in DDA.
%   }
%   \label{appendixTab:diffusionrefinementrange}
%   \begin{center}
%    		\adjustbox{max width=\linewidth}{
%    			\renewcommand\arraystretch{1.15}
%    			\begin{tabular}{ll|ccc}
%    				& $D=4$
%    				% & RedNet-26
%    				& ResNet-50
%    				& Swin-T
%    				& ConvNeXt-T
%    				\\
%    				\midrule
%    				% \multirow{3}{*}{(a) trans}
%    				& 3
%    				% & 33.2     
%                     & 34.3     & 40.5      & 38.8
%    				\\
%    				\rowcolor{lightgray} (a) elastic transformation & 6
%    				% & 34.3     
%                     & 35.6     & 40.5      & 38.4
%    				\\
%    				& 9
%    				% & 33.9     
%                     & 34.6     & 38.4      & 36.7
%    				\\
%    				\midrule
%    				% \multirow{3}{*}{(b) blur}
%    				& 3
%    				% & 16.1     
%                     & 16.6     & 26.8      & 22.6
%    				\\
%    				\rowcolor{lightgray} (b) glass blur & 6
%    				% & 14.5     
%                     & 15.3     & 23.6      & 19.7
%    				\\
%    				& 9
%    				% & 13.4     
%                     & 14.0     & 20.4      & 17.1
%    				\\
%    				\midrule
%    				% \multirow{3}{*}{(c) noise}
%    				& 3
%    				% & 24.8     
%                     & 26.6     & 38.8      & 34.4
%    				\\
%    				\rowcolor{lightgray} (c) shot noise & 6
%    				% & 36.4     
%                     & 37.2     & 42.9      & 39.8
%    				\\
%    				& 9
%    				% & 36.4     
%                     & 37.0     & 41.2      & 38.6
%    				\\
%    				\bottomrule
%    			\end{tabular}
%    		}
%     \end{center}
% \end{table}
