# Supplementary material for: Diffusion Model Driven Test-Time Image Adaptation for Robust Skin Lesion Classification
Source: arXiv:2405.11289 source file (2024-05-18)
Supplement: Supplementary file 9 [file appendix_scalingfactor.tex]

\begin{table}[t]
  \caption{
	\textbf{Ablation on choices of scaling factor $D$ with fixed $\boldsymbol{w}$.} 
	Our default hyper-parameter is in the shadow row.
	The empirical results confirm the choice of hyper-parameters in DDA.
  }
  \label{appendixTab:diffusionscalingfactor}
  \begin{center}
   		\adjustbox{max width=\linewidth}{
   			\renewcommand\arraystretch{1.15}
   			\begin{tabular}{ll|ccc}
   				& $\boldsymbol{w}=6$
   				% & RedNet-26
   				& ResNet-50
   				& Swin-T
   				& ConvNeXt-T
   				\\
   				\midrule
   				% \multirow{3}{*}{(a) trans}
   				& 2
   				% & 29.0    
                    & 22.2    & 29.9     & 31.2
   				\\
   				\rowcolor{lightgray} (a) elastic transformation & 4
   				% & 34.3    
                    & 32.3    & 38.9     & 41.2
   				\\
   				& 8
   				% & 33.0    
                   & 41.6     & 45.2  & 48.0
   				\\
   				\midrule
   				% \multirow{3}{*}{(b) blur}
   				& 2
   				% & 13.8    
                    & 9.5      & 13.4  & 14.9
   				\\
   				\rowcolor{lightgray} (b) glass blur & 4
   				% & 14.5    
                    & 12.0     & 17.6  & 19.9
   				\\
   				& 8
   				% & 20.4   
                    & 19.7     & 26.0  & 29.8  
   				\\
   				\midrule
   				% \multirow{3}{*}{(c) noise}
   				& 2
   				% & 25.3    
                    & 50.4     & 54.5  & 58.7
   				\\
   				\rowcolor{lightgray} (c) shot noise & 4
   				% & 36.4    
                    & 48.7     & 53.2  & 57.3
   				\\
   				& 8
   				% & 28.3    
                    & 40.4     & 44.6  & 48.7 
   				\\
   				\bottomrule
   			\end{tabular}
   		}
    \end{center}
\end{table}

% \begin{table}[t]
%   \caption{
% 	\textbf{Ablation on choices of scaling factor $D$ with fixed $M$.} 
% 	Our default hyper-parameter is in the shadow row.
% 	The empirical results confirm the choice of hyper-parameters in DDA.
%   }
%   \label{appendixTab:diffusionscalingfactor}
%   \begin{center}
%    		\adjustbox{max width=\linewidth}{
%    			\renewcommand\arraystretch{1.15}
%    			\begin{tabular}{ll|ccc}
%    				& $\boldsymbol{w}=6$
%    				% & RedNet-26
%    				& ResNet-50
%    				& Swin-T
%    				& ConvNeXt-T
%    				\\
%    				\midrule
%    				% \multirow{3}{*}{(a) trans}
%    				& 2
%    				% & 29.0    
%                     & 30.2    & 37.6     & 35.7
%    				\\
%    				\rowcolor{lightgray} (a) elastic transformation & 4
%    				% & 34.3    
%                     & 35.6    & 40.5     & 38.4
%    				\\
%    				& 8
%    				% & 33.0    
%                     & 33.4    & 36.3     & 34.8
%    				\\
%    				\midrule
%    				% \multirow{3}{*}{(b) blur}
%    				& 2
%    				% & 13.8    
%                     & 14.0    & 22.8     & 19.2
%    				\\
%    				\rowcolor{lightgray} (b) glass blur & 4
%    				% & 14.5    
%                     & 15.3    & 23.6     & 19.7
%    				\\
%    				& 8
%    				% & 20.4   
%                     & 20.6    & 24.4    & 22.6
%    				\\
%    				\midrule
%    				% \multirow{3}{*}{(c) noise}
%    				& 2
%    				% & 25.3    
%                     & 28.6    & 41.5     & 37.2
%    				\\
%    				\rowcolor{lightgray} (c) shot noise & 4
%    				% & 36.4    
%                     & 37.2    & 42.9     & 39.8
%    				\\
%    				& 8
%    				% & 28.3    
%                     & 28.7    & 31.9     & 30.2
%    				\\
%    				\bottomrule
%    			\end{tabular}
%    		}
%     \end{center}
% \end{table}
